# Supplementary material for: Non-linear optical spectroscopy and two-photon excited fluorescence spectroscopy reveal the excited states of fluorophores embedded in beetle's elytra
Source: arXiv:1801.07639 source file (2018-01-23)
Supplement: Supplementary file 1 [file Mouchet_SI_submitted.pdf]

# Supplementary Information

# Non-linear optical spectroscopy and two-photon excited fluorescence spectroscopy reveal the excited states of fluorophores embedded in beetle's elytra

Sébastien R. Mouchet, Charlotte Verstraete, Dimitrije Mara, Stijn Van Cleuvenbergen, Ewan D. Finlayson, Rik Van Deun, Olivier Deparis, Thierry Verbiest, Bjorn Maes, Pete Vukusic, and Branko Kolaric

Supplementary Information 1:

Morphological characterisation

The electron microscopy analyses of the morphology of the scales covering the elytra were performed with a FEI (Hillsboro, OR, USA) Nova Nanolab 200 Dual-Beam scanning electron microscope (SEM). Elytra were cut into 5x5$^2$ size pieces and fixed on the sample mount with conducting tape. 20-nm thick platinum layer was sputter-coated on the samples. The focused-ion beam (FIB) of the dual-beam SEM was used to cut sharply and properly the samples.

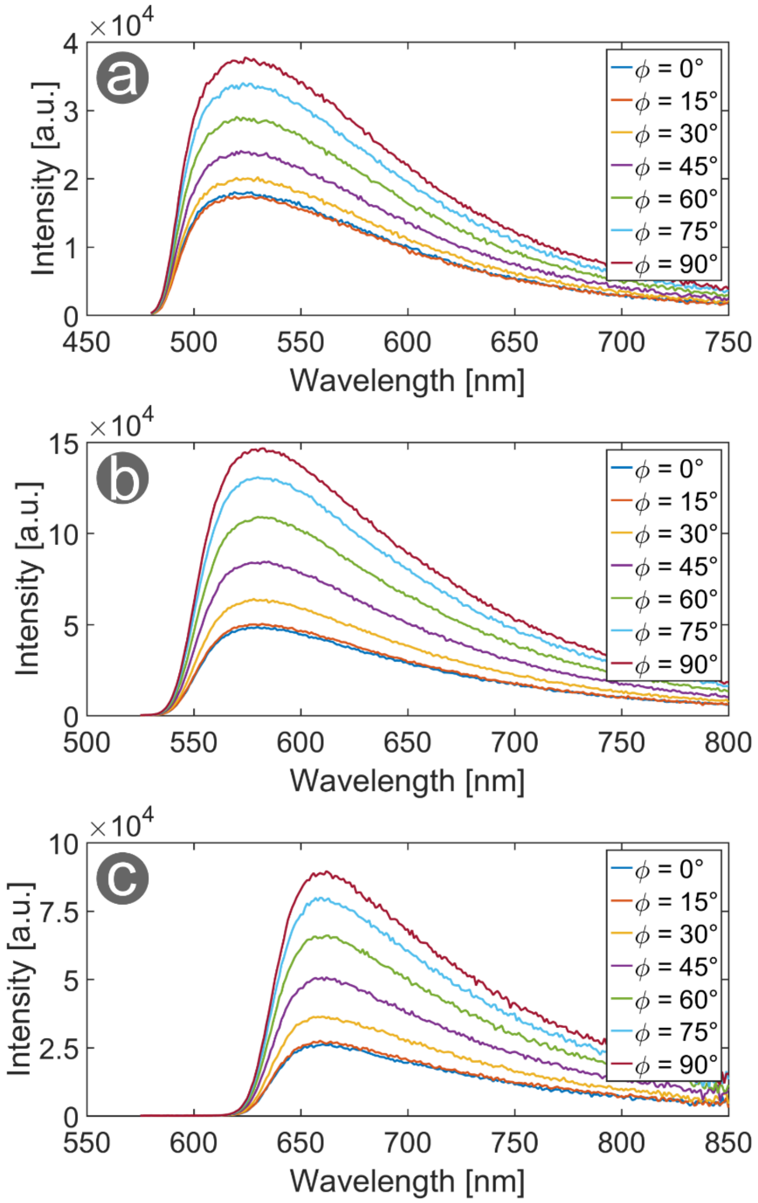


Supplementary Figure 1: **OPEF response of *H. coerulea*'s elytra.** (a-c) The OPEF emission spectra from the fluorophores embedded within the beetle's photonic structure depend strongly on the linear polarisation states. ϕ is the angle of the rotating polariser. The excitation wavelengths are equal to (a) 450 nm, (b) 500 nm and (c) 550 nm, respectively.

| $\lambda_{em}$ (nm) | τ (ns) in dry state | τ (ns) in wet state |
|---|---|---|
| 466 | 3.9<br>0.79 | 1.4 |
| 546 | 1.9 | 1.4 |

Supplementary Table 1: **Decay times τ of the fluorophores embedded within the male *H. coerulea* beetle's photonic structures.** Measurements were performed in both dry and wet states for emission wavelengths $\lambda_{em}$ located inside (466 nm) and outside (546 nm) the structure PhBG [1]. The incident 376-nm light beam and the emitted light formed 45° angles at either side of the direction normal to the sample surface.

Supplementary Movie 1: **3D reconstruction of the TPEF signal from *H. coerulea*'s elytra.** The strong TPEF response from the elytra of the male *H. coerulea* with a 900-nm excitation light and a 15x magnification was used in order to perform a 3D reconstruction of the scales covering these elytra.

**Supplementary References**

1. S. R. Mouchet, M. Lobet, B. Kolaric, A. M. Kaczmarek, R. Van Deun, P. Vukusic, O. Deparis and E. Van Hooijdonk, "Controlled fluorescence in a beetle's photonic structure and its sensitivity to environmentally induced changes," Proc. R. Soc. London B Biol. Sci. 283, 20162334, 2016.
